# Supplementary material for: Neighborhood-based Hypergraph Core Decomposition
Source: arXiv:2301.06426 source file (2023-04-09)
Supplement: Supplementary file 1 [file appendix.tex]

\section{appendix}
\label{appendix}
\subsection{Top-down algorithm}
\label{subsec:top-down}

 The idea is to give a local upper bound based on the upper bound derived from weak definition of sub-hypergraph (\cref{eq:wk-subhg}).

\begin{definition}[weak nbr-k-core]
The weak neighborhood k-core $H^w_k := (V_k,E^w[V_k]$ of a hypergraph $H = (V,E)$ is the maximal weak sub-hypergraph such that every vertex $u \in V_k$ has at least $k$ neighbors in $H^w_k$. The weak core-index $core^w(v)$ of a vertex $v$ is the largest $k$ for which the weak k-core $H^w_k$ contains $v$.
\end{definition}
\begin{lemma}[local upper bound]
% \label{lem:localUB}
For any vertex $v$, its neighborhood core-index $core(v) \leq core^w(v)$.
\end{lemma}
\begin{proof}
% Proof by induction on core number $k = core(v)$.
% \paragraph{Base case (k=1):} Need to show that for any vertex $v$ with $core(v) = 1$, $core^w(v) \geq 1$.
% \paragraph{Induction:} Assume for any vertex $v$ with $core(v) = k$ $core^w(v) \geq k$. Need to show that for any vertex $u$ with $core(u) = k+1$, $core^w(u) > k+1$.

Let $H_k = (V_k,E[V_k])$ be the strong nbr-k-core of an arbitrarily chosen vertex $v$. By definition of strong sub-hypergraph $E[V_k] \subseteq E$.

Let $H^w[V_k] = (V_k,E^w[V_k])$ be the weak sub-hypergraph induced by $V_k$. Let $\abs{N^w_{V_k}(v)}$ be the number of neighbors of $v$ in the weak-subhypergraph $H^w$.

Every $e \in E[V_k]$ has the property that $e \in E$ and $e = e \cap V_k \neq \phi$, otherwise $e$ would not be an edge in $H_k$. Thus $e \in E^w[V_k]$ by definition of weak-subhypergraph and consequently $E[V_k] \subseteq E^w[V_k]$. Since $N_{V_k}(v):= \cup_{e_i \ni v \land e_i \in E[V_k]} e_i$ and $N^w_{V_k}:= \cup_{e_i \ni v \land e_i \in E^w[V_k]} e_i$, $N_{V_k}(v) \subseteq N^w_{V_k}(v)$. It follows that for any $u \in V_k$, $k \leq \abs{N_{V_k}(u)} \leq \abs{N^w_{V_k}(u)}$.

Since ever vertex $u \in V_k$ has at least $k$ neighbors in the weak-subhypergraph $H^w[V_k]$ and the weak nbr-k-core is maximal among such weak-subhypergraphs, weak nbr-k-core must contain hyperedges from $H^w[V_k]$.

Thus $v$ must be present in the weak nbr-k-core. It follows that the weak nbr-core index of $v$ must be at least $k$. Since $v$ was arbitrarily chosen, for any $v \in V$, $core(v) \leq core^w(v)$.

% certainly this property will hold for the maximal weak-subhypergraph containing $v$ as well.

% Suppose $I^w(v)$ be the subset of edges in $E^w[S_k]$ incident on $v$.

% \textbf{Case 1 ($I^w(v) \subseteq E$):}

% \textbf{Case 2 ($I^w(v) \not\subseteq E$):}

\end{proof}

{\color{red} Unlike graphs, the following does not hold in hypergraphs.
\begin{lemma}
% \label{lem:sufficiency_of_localUB}
Let $V[i] = \{u \in V: \mathbf{UB_2}(u) \geq i\}$. For every vertex $v \in V$ with $core(v)>=i$, its nbr $k$-core $core_{V[i]}(v)$ is computable from $H[V[i]]$.
\end{lemma}
}
\paragraph{Computation of Local Upper Bound}~\Cref{alg:localUB}
{\color{blue} To do: Describe with an Example.}

\paragraph{The algorithm LLB-LUB.}
Top-down computation by dividing $[LB_1,UB_1]$ into disjoint partitions. Innermost core would be computed first to avoid repeated bucket updates+nbr-computation of innermost core-vertex.

{\color{blue} To do: Describe with Examples.}

% \begin{algorithm}[!htb]
% \begin{algorithmic}[1]
% \caption{\label{alg:localUB2}Local Upper Bound Algorithm\#1}
% \Require Hypergraph $H = (V,E)$
% \Ensure Upper-bounds $\mathbf{UB_2}[u]$ for each vertex $u \in V$
% % \ForAll {$i \in [\abs{V}]$}
%     \State Initialise bucket $B[i] \gets \phi, \forall i \in [1,\abs{V}]$
% % \EndFor
% \ForAll {$u \in V$}
%     \State Compute $N_V(u)$
%     \State $B[\abs{N_V(u)}] \gets B[\abs{N_V(u)}] \cup \{u\}$
% \EndFor
% \ForAll {$k = 1,2,\ldots, \abs{V}$}
%     \While{$B[k] \neq \phi$}
%         \State Remove a vertex $v$ from $B[k]$
%         \State $\mathbf{UB_2}[v] \gets k$
%         \ForAll{$u \in N_V(v)$}
%             \State Compute $N_{V}(u)$
%             \State Move $u$ to $B[\max{\left(\abs{N_{V}(u)} - 1, k \right)}]$
%         \EndFor
%         \State  Compute weak sub-hypergraph $H^w[V \setminus \{v\}]$
%         \State $H \gets H^w[V \setminus \{v\}]$
%     \EndWhile
% \EndFor
% \end{algorithmic}
% \end{algorithm}

\begin{algorithm}[!htb]
\begin{algorithmic}[1]
% \caption{\label{alg:localUB} \textbf{ComputeLUB}: Local Upper Bound Computation}
\Require Hypergraph $H = (V,E)$
\Ensure Upper-bounds $\mathbf{UB_2}[u]$ for each vertex $u \in V$
% \ForAll {$i \in [\abs{V}]$}
    \State Initialise bucket $B[i] \gets \phi, \forall i \in [1,\abs{V}]$
% \EndFor
\ForAll {$u \in V$}
    \State Compute $N_V(u)$
    \State $B[\abs{N_V(u)}] \gets B[\abs{N_V(u)}] \cup \{u\}$
    \State Initialise bucket index $Idx[u] \gets \abs{N_V(u)}$
\EndFor
\ForAll {$k = 1,2,\ldots, \abs{V}$}
    \While{$B[k] \neq \phi$}
        \State Remove a vertex $v$ from $B[k]$
        \State $\mathbf{UB_2}[v] \gets k$
        \ForAll{$u \in N_V(v)$}
            \If{$u \notin \mathbf{UB_2}$}
                \State Move $u$ to $B[\max{\left(Idx[u] - 1, k \right)}]$
                \State $Idx[u] \gets \max{\left(Idx[u] - 1, k \right)}$
            \EndIf
        \EndFor

    \EndWhile
\EndFor
\State return $\mathbf{UB_2}$
\end{algorithmic}
\end{algorithm}

\begin{algorithm}[!htb]
\begin{algorithmic}[1]
% \caption{\label{alg:ivalgenerator} \textbf{IntervalGen:} Partitioning local lower bound and upper bound into disjoint intervals}
\Require Hypergraph $H = (V,E)$, Local Upper Bounds $\mathbf{UB}_2$, Local Lower Bounds $\mathbf{LB}_2$, parameter $s \in \mathbb{Z}^+$
\Ensure Array of Intervals $I$
\State $MINLLB = \min_{u \in V} \mathbf{LB}_2(u) $
\State $UBset =  \{ \mathbf{UB}_2(u): u \in V \} \cup \{MINLLB-1\}$
\State Sort $UBset$ in descending order.
\State Initialize $i \gets s$
\State Initialize $I \gets [~]$
\While{$i < UBset.size()$}
    \State Insert $[UBset[i] + 1, UBset[i - s]]$ to $I$
    \If{$ i+s \geq UBset.size() \land i \neq UBset.size() - 1$}
        \State Insert $[UBset[UBset.size()-1] + 1, UBset[i]]$ to $I$
    \EndIf
    \State $i \gets i + s$

\EndWhile
\State return $I$
\end{algorithmic}
\end{algorithm}

\begin{algorithm}[!htb]
\begin{algorithmic}[1]
\caption{
% \label{alg:Improvedalg2} 
\textbf{LLB-LUB:} Local lower bound and upper bound based nbr-k-core decomposition}
\Require Hypergraph $H = (V,E)$, parameter $s>0$
\Ensure Core index $c[u]$ for each vertex $u \in V$
\State Initialize bucket $B[i] \gets \phi, \forall i \in [1,\abs{V}]$
\State Initialize $setLB[u] \gets True, \forall u \in V$
\State Initialize bucket index $Idx[u] \gets -1, \forall u \in V$
\State Local upper bound $\mathbf{UB}_2 \gets \textbf{ComputeLUB}(H)$
\State Local lower bound $\mathbf{LB}_2$.
\State Descending set of intervals $I \gets \textbf{IntervalGen}(H,\mathbf{UB}_2,\mathbf{LB}_2,s)$
\For {$(k_{min}, k_{max}) \in I$}
    \State  $V[k_{min}] \gets \{u \in V: \mathbf{UB}_2(u) \geq k_{min}\}$
    \For{$u \in V[k_{min}]$}
        \State $Idx[u] \gets \max\left(k_{min}-1, \mathbf{LB}_2(u),c[u]\right)$
        \State $B[Idx[u]] \gets B[Idx[u]] \cup \{u\}$
        \State $setLB(v) \gets True$

    \EndFor
    \State Compute sub-hypergraph $H[V[{k_{min}}]]$
    \ForAll{$k \gets k_{min}-1,k_{min},\ldots, k_{max}$}
        \While{$B[k] \neq \phi$}
        \State Pick and remove $v$ from $B[k]$
        \If{$setLB(v)$}
            \State Compute $N_{V[k_{min}]}(v)$
            \State $Idx[v] \gets \abs{N_{V[{k_{min}}]}(v)}$
            \State $B[Idx[v]] \gets B[Idx[v]] \cup \{v\}$
            \State $setLB(v) \gets False$
        \Else
            \State $c[v] \gets k$
            \State $setLB(v) \gets True$
            \State $V'[k_{min}] \gets V[k_{min}] \setminus \{v\}$
            \For{$u \in N_{V[k_{min}]}(v)$}
                \State Compute $N_{V'[k_{min}]}(u)$
                \State Move $u$ to $B[\abs{N_{V'[k_{min}]}(u)}]$
                \State $Idx[u] \gets \abs{N_{V'[k_{min}]}(u)}$
            \EndFor
            \State $V[k_{min}] \gets V'[k_{min}]$
        \EndIf
        \EndWhile
    \EndFor
\EndFor
\State return $c$
\end{algorithmic}
\end{algorithm}

\textbf{Proof of Correctness.}

\textbf{Complexity analysis. }

\subsection{Exact algorithm for finding volume-densenst sub-hypergraph}
We use binary search to find the volume-densest sub-hypergraph. For each candidate value $  \frac{\sum_{u\in V}\abs{N(u)}}{\abs{V}} \leq \eta \leq \sum_{u \in V} \abs{N(u)}$ , we define a flow network $G_\eta$ , which is a directed graph with edge-capacities, and has source $s$
and sink $t$. The set of nodes in $G_\eta$ is $\{s\}\cup\{t\}\cup V \cup E$. The set of edges are defined as following (see~\cref{fig:aux}):

\begin{itemize}
    \item For all $u \in V$, the capacity $c(s,u)$ of edge $(s,u)$ is $N(u)$.
    \item For all $u\in V$, the capacity $(c(u,t)$ of edge $(u,t)$ is $\eta$.
    \item For all edge $e \in E$ and vertex $u \in V$, the capacity $c(u,e)$ of edge $(u,e)$ is $(\abs{e}-1)$ and the capacity $c(e,u)$ of edge $(e,u)$ is $\infty$.
\end{itemize}
Thus $G_\eta$ has $\abs{V}+\abs{E}+2$ vertices and $O(\abs{V}+\abs{E})$ edges and can be constructed in $O(\abs{V}+\abs{E})$ time. Note that, all capacities are non-negative.

\begin{figure}[!t]
    \centering
    \includegraphics[width=0.4\textwidth]{figures/auxiliary.pdf}
    \caption{Auxiliary graph $G_\eta$}
    \label{fig:aux}
\end{figure}

\begin{lemma}
\label{lem:maxflow}
The maximum flow from $s$ to $t$ in $G_\eta$ is strictly less than $N(V):= \sum_{u \in V} \abs{N(u)}$ if and only if $\rho^N[S^*] > \eta$.
\end{lemma}
\begin{proof}
Note that we always have max-flow at most $N(V):= \sum_{u \in V} \abs{N(u)}$ since there is an st-cut $(\{s\},\{V,E,t\})$ of capacity $N(V)$.

Suppose we compute the max-flow from $s$ to $t$ in $G_\eta$ and find a minimum st-cut as $(\{s\} \cup V_1 \cup E_1, \{t\} \cup V_2 \cup E_2)$, where $V_2 = V \setminus V_1$, $E_2 = E\setminus E_1$, then we have (where $cut(A, B)$ is the total capacities of edges from $A$ to $B$):

% \begin{equation*}
    \begin{align}
    \label{eq:maxflow}
        \text{max-flow}(s,t;G_\eta) &= \text{cut}(\{s\}\cup V_1 \cup E_1,\{t\}\cup V_2 \cup E_2) \notag\\
        & = \text{cut}(s,V_2) + \text{cut}(V_1,E_2) +   \text{cut}(E_1,V_2) + \text{cut}(V_1,t) \notag\\
        & = N(V_2) + \text{cut}(V_1,E_2) +   \text{cut}(E_1,V_2) + \eta \abs{V_1}
    \end{align}
% \end{equation*}

Now, $\text{cut}(E_1,V_2) = 0$ since otherwise $\text{cut}(E_1,V_2) = \infty$; this implies that for any $e$ such that $e \cap V_2 \neq \phi$  can not be in $E_1$.

On the other hand, since $(\{s\} \cup V_1 \cup E_1, \{t\} \cup V_2 \cup E_2)$ is a minimum st-cut, if there is an edge $e \subseteq V_1$ such that $e \in E_2$, then we can strictly reduce the cut by moving $e$ from $E_2$ to $E_1$. This implies that $E[V_1] = E_1$ and $E \setminus E[V_1] = E_2$.

It follows that
\begin{equation*}
    \begin{split}
    \text{cut}(V_1,E_2) &= \text{cut}(V_1,E) - \text{cut}(V_1,E[V_1]) \\
    &= \sum_{u \in V_1} \abs{N(u)} - \sum_{u \in V_1} N_{V_1}(u) \\
    &= N(V_1) - N_{V_1}(V_1)
    \end{split}
\end{equation*}

From~\cref{eq:maxflow} it follows that,
\begin{align*}
    \text{max-flow}(s,t;G_\eta) &= N(V_2) + N(V_1) - N_{V_1}(V_1) + \eta\abs{V_1} \\
    &= N(V) - \abs{V_1}(\frac{N_{V_1}(V_1)}{\abs{V_1}} - \eta)\\
    &= N(V)- \abs{V_1}(\rho^N[V_1] - \eta)
\end{align*}

If $\text{max-flow}(s,t;\eta) < N(V)$, it follows that $\rho^N[V_1] > \eta$. Thus the true densest volume density $\rho^N[S^*] \geq \rho^N[V_1] > \eta$.

Conversely, if $\exists~V_1 \subseteq V$ such that $\rho^N[V_1] > \eta$,  by taking $V_2 := V\setminus V_1$, $E_1 := E[V_1]$ and $E_2 := E\setminus E_1$, the cut $(\{s\} \cup V_1 \cup E_1, \{t\}\cup V_2 \cup E_2)$ has capacity $N(V) - \abs{V_1}(\rho^N[V_1] - \eta) < N(V)$. It follows that the max-flow $\text{max-flow}(s,t;\eta) < N(V)$.

\end{proof}

\begin{lemma}[Density gap lemma]
\label{lem:gap}
The density gap $\Delta$ defined as
$\Delta := \abs{\rho^N[S_1] - \rho^N[S_2]}$ between two sub-hypergraphs $(S_1,E[S_1])$ and $(S_2,E[S_2])$ of distinct volume-densities is at least $\frac{1}{2\abs{V}^2}$.
\end{lemma}
\begin{proof}
Since for $S_1,S_2 \subseteq V$, $\rho^N[S_1] \neq \rho^N[S_2]$, it follows that
\begin{align}
\label{eq:dgap}
    \Delta := \abs{\rho^N[S_1] - \rho^N[S_2]} \notag\\
            &= \abs{ \frac{N(S_1)}{\abs{S_1}} - \frac{N(S_2)}{\abs{S_2}} } \notag\\
            &= \abs{\frac{\abs{S_2}N(S_1) - \abs{S_1}N(S_2)}{\abs{S_1}\abs{S_2}}}
\end{align}
\paragraph{Case 1 ($\abs{S_1} = \abs{S_2}$): }
Since both $\abs{S_1}$ and $\abs{S_2}$ is at most $\abs{V}$ and $N(S_1) \neq N(S_2)$ due to the fact that $(S_1,E[S_1])$ and $(S_2,E[S_2]$ have distinct volume-densities, it follows from~\cref{eq:dgap} that $\Delta = \abs{\frac{N(S_1) - N(S_2)}{\abs{S_1}}} \geq \frac{1}{\abs{V}} > \frac{1}{2\abs{V}^2}$.

\paragraph{Case 2 ($\abs{S_1} \neq \abs{S_2}$): }  Without loss of generality, let us assume $\abs{S_1} > \abs{S_2}$.
Since $\abs{S_1} - \abs{S_2} \leq \abs{V}$, it follows that $\abs{S_1} \leq \abs{S_2} + \abs{V} \leq 2\abs{V}$. Thus $\abs{S_1}\abs{S_2} \leq 2\abs{V}^2$. From~\cref{eq:dgap} it follows that,
\begin{align}
\label{eq:gap2}
    \Delta &\geq \frac{\abs{\abs{S_2}N(S_1) - \abs{S_1}N(S_2)}}{2\abs{V}^2}
\end{align}

% If $N(S_1) = N(S_2)$, since $\abs{S_2}$ and $\abs{S_1}$ must differ by at least $1$ vertex, $\Delta \geq \frac{1}{2\abs{V}^2}$. If $N(S_1) \neq N(S_2)$,
Since $(S_1,E[S_1])$ and $(S_2,E[S_2])$ have distinct volume densities the numerator of~\cref{eq:gap2} can not be zero. Since $\abs{S_1}$, $\abs{S_2}$, $N(S_1)$ and $N(S_2)$ are all integers, the numerator of~\cref{eq:gap2} must be at least $1$. It follows that $\Delta \geq \frac{1}{2\abs{V}^2}$.
\end{proof}
\Cref{lem:maxflow} and~\Cref{lem:gap} leads to the following theorem:-
\begin{theorem}
If $H'$ is a sub-hypergraph of $H$ with volume density $\rho^N[H']$ and no sub-hypergraph of $H$ has volume-density greater than or equal to $\rho^N[H'] + \frac{1}{2\abs{V}^2}$, $H'$ is a sub-hypergraph of maximal volume-density.
\end{theorem}
The theorem gives us a termination condition for binary search for densest sub-hypergraph. We can now describe our algorithm:-

\paragraph{The algorithm ...}

\begin{algorithm}[!htb]
\caption{Exact volume-densest sub-hypergraph}
\label{alg:exact}
\begin{algorithmic}[1]
\Require Hypergraph $H = (V,E)$
\Ensure Hypergraph $H[S^*]$
\State $lower \gets \frac{\sum_{u \in V} \abs{N(u)}}{\abs{V}}$
\State $upper \gets \sum_{u \in V} \abs{N(u)}$
\State $\Delta \gets \frac{1}{2\abs{V}^2}$
\While{$upper - lower \geq \Delta$}
\State $\eta \gets \frac{lower + upper}{2}$
\State Construct auxiliary graph $G_\eta$.
\State Find $\text{max-flow}(s,t; G_\eta) := \text{cut}(V_\eta,E_\eta)$
\If{ $\text{cut}(V_\eta,E_\eta) < upper$}
\State $lower \gets \eta$
\State $S^* \gets V_\eta \cap V$ \Comment{$S^*$ is the candidate vertices s.t. $\rho^N[S^*] > \eta$}
\Else
\State $upper \gets \eta$ \Comment{$\forall S\subseteq V, \rho^N[S] \leq \eta$ and $\rho^N[S^*] \leq \eta$}
\EndIf
\EndWhile
\State \textbf{return} $H[S^*]$
\end{algorithmic}
\end{algorithm}

We illustrate the pseudocode in~\Cref{alg:exact}.

% \paragraph{Goldberg-type~\cite{goldberg} max-flow-based argument}

% See~\cref{fig:exact-algorithm1},~\cref{fig:exact-algorithm2} and~\cref{fig:exact-algorithm3}

% \begin{figure}
%     \centering
%     \includegraphics[width=0.35\textwidth]{figures/exact-algorithm1.pdf}
%     \includegraphics[width=0.35\textwidth]{figures/exact-algorithm2.pdf}
%     \caption{Auxiliary graph construction and showing that if max-flow from s to t is at most $\sum_{u \in V} N(u)$, there exists a subset $V_1 \subset V$ (derived from min-cut) that is denser than our prior `guess' ($\eta$) of density.}
%     \label{fig:exact-algorithm1}
% \end{figure}

% \begin{figure}
%     \centering
%     \includegraphics[width=0.4\textwidth]{figures/exact-algorithm3.pdf}
%     \includegraphics[width=0.4\textwidth]{figures/exact-algorithm4.pdf}
%     % \caption{Exact}
%     \caption{\label{fig:exact-algorithm2} The lower bound for the gap between a pair of distinct volume-density values.}
% \end{figure}

% \begin{figure}
%     \centering
%     \includegraphics[width=0.4\textwidth]{figures/exact-algorithm5.pdf}
%     \includegraphics[width=0.4\textwidth]{figures/exact-algorithm6.pdf}
%     % \caption{Exact}
%     \caption{\label{fig:exact-algorithm3} Turning the density gap and max-flow based analysis on auxiliary graph into a binary-search based exact algorithm for computing volume-densest sub-hypergraph.}
% \end{figure}

\subsection{deg-based core decomposition algorithm}
Pseudocode for the sake of our experimental analysis:~\cref{alg:degcore}
\begin{algorithm}[!htb]
\begin{algorithmic}[1]
\caption{\label{alg:degcore}Naive deg-k-core decomposition}
\Require Hypergraph $H = (V,E)$
\Ensure Core index $c[u]$ for each vertex $u \in V$
% \ForAll{$i \in [\abs{V}]$}
\State Initialise dictionary $B \gets \{\}$
% \EndFor
\ForAll {$u \in V$}
    \State Compute $d_V(u)$ \Comment{degree($u$) in $H=(V,E)$}
    \If{$d_V(u) \notin B$}
    \State $B[d_V(u)] = \{u\}$
    \Else
    \State $B[d_V(u)] \gets B[d_V(u)] \cup \{u\}$
    \EndIf
\EndFor
\State Compute maximum of degrees $d_{max} \gets \max_{u \in V} d_V(u)$
\ForAll {$k = 1,2,\ldots, d_{max}$}
    \While{$B[k] \neq \phi$}
        \State Remove a vertex $v$ from $B[k]$
        \State $c[v] \gets k$
        \State $V' \gets V \setminus \{v\}$
        \State Compute sub-hypergraph $H[V']$
        \ForAll{$u \in N_V(v)$}
            \State Compute $d_{V'}(u)$ \Comment{degree($u$) in $H[V']$}
            \State Move $u$ to $B[\max{\left(\abs{d_{V'}(u)},k \right)}]$
        \EndFor
        \State $V \gets V'$
    \EndWhile
\EndFor
\end{algorithmic}
\end{algorithm}

\subsection*{Defining $k$-core from a stronger notion of vertex degree\cite{ramadan2004hypergraph}.} One can adopt a stronger definition of degree by counting only those incident hyperedges that are maximal, meaning, hyperedges that are not subset of other hyperedges.

\emph{maximal degree} $d^{m}_H(v)$ of a vertex $v$ in hypergraph $H = (V,E)$ is the number of maximal hyperedges incident on $v$. A hyperedge is maximal if there is no hyperedge (except itself) containing it.
Mathematically,

$ d^m_H(v) := \abs{\{e \in E: v \in e \land  \nexists_{e'\in E} e' \supset e\}}$

\emph{$k$-core of a hypergraph~\cite{ramadan2004hypergraph}}
The $k$-core $H_k$ of a hypergraph $H$ is a maximal induced sub-hypergraph $H_k$ such that every vertex $v$ in $H_k$ has maximal degree at least $k$.

\subsection*{vertex-cover of a hypergraph.}

\paragraph{Minimum-weighted vertex cover.} Given a vertex-weighted hypergraph $H = (V,E,W:V \times V \rightarrow Z^+)$, a minimum-weighted vertex cover of $H$ is a subset $C \subset V$ of vertices such that
\begin{enumerate}
    \item every hyperedge is incident on some vertex $v \in C$ (cover property), and
    \item the sum of vertex weights $\sum_{v \in C} W(v)$ is the smallest (minimality property).
\end{enumerate}

\textbf{TO DO: Figures}

\subsubsection*{Vertex-cover: Related Works}
\paragraph{Application/Modelling in nature.}
Ramadan et al.~\cite{ramadan2004hypergraph} argues that the problem of selecting bait proteins from protein complex data can be modelled as computing minimum-weighted vertex cover of the protein complex hypergraph.

One of the problems with large-scale proteomic techniques is the relatively lower reliability of the experimental results. For instance, in the Cellzome experiment a set of bait proteins in the yeast is required to identify multi-protein complexes via a number of lab experiments. The outcome of the experiment is a dataset of protein complexes identified from various bait proteins. Each complex is identified by the proteins it contains. In such experiments, the problem of selecting bait proteins from a protein complex hypergraph can be useful in two scenarios-

Firstly, One may wish to improve the reliability of the data by finding bait proteins computationally from protein complex hypergraph of an earlier experiment and then repeat the experiments using the newly derived bait proteins. Lastly, one may wish to use one organism as a model to identify the protein complexes in a related organism.

\paragraph{Algorithmic in nature.} Ramadan et al.~\cite{ramadan2004hypergraph} proposed a greedy algorithm to compute approximate minimum-weighted vertex cover from protein complex hypergraph.

\paragraph{Existing approximation bounds.} Ramadan et al.~\cite{ramadan2004hypergraph} does not derive any approximation guarantee.

\subsection*{k-connectivity of a hypergraph.}
\subsubsection*{k-connectivity: Related Works}

\subsection*{Hypergraph clustering coefficient.}
\subsubsection*{Clustering coefficients: Related Works}

\subsection{LP based exact algorithm}
We give an exact algorithm by showing that densest subgraph finding problem is equivalent to finding an optimal solution to a Linear Programming problem.

See~\cref{fig:lp} for the formulation.
See~\cref{fig:lem1} and~\cref{fig:lem2} for the proof of two lemmas leading to the theorem in~\cref{fig:equivthm}.

\begin{figure}[!htb]
    \centering
     \begin{minipage}{0.4\linewidth}
        \includegraphics[width=\linewidth]{prooffigs/LP.pdf}
        \caption{\label{fig:lp}LP formulation}
    \end{minipage}
    \begin{minipage}{0.4\linewidth}
        \includegraphics[width=\linewidth]{prooffigs/Proof1.pdf}
        \caption{\label{fig:lem1}Proof of Lemma 1}
    \end{minipage}
\hspace{0.5cm}
    \begin{minipage}{0.4\linewidth}
      \includegraphics[width=\linewidth]{prooffigs/Proof2.pdf}
      \caption{Proof of Lemma 2.}
        \label{fig:lem2}
    \end{minipage}
    \begin{minipage}{0.4\linewidth}
      \includegraphics[width=\linewidth]{prooffigs/LP_theorem.pdf}
      \caption{The theorem.}
        \label{fig:equivthm}
    \end{minipage}
\end{figure}

\subsection{Local algorithm theories}
{\color{red} This operator does not take into account hyperedge constraint locally. Meaning, if a vertex $i$ and a neighbour $x$ are in a subgraph (say in $k$-core), any edge between $i-x'$ are also in a subgraph ($k$. But in a hypergraph, this is not necessarily true.}

\begin{definition}[$\mathcal{H}$-operator~\cite{eugene15}]
Let $\mathcal{H}$ be an operator acting on a finite set of reals $\{x_1,x_2,\ldots,x_n\}$ and returns an integer $y = \mathcal{H}\left(x_1,x_2,\ldots,x_n\right) > 0$, where $y$ is the maximum integer such that there exist at least $y$ elements in $\{x_1,x_2,\ldots,x_n\}$, each of which is at least $y$.
\end{definition}

\begin{example}[$H$-operator]
$\mathcal{H}(1,1,1,1) = 1$\\
$\mathcal{H}(1,1,1,2) = 1$\\
$\mathcal{H}(1,1,2,2) = 2$\\
$\mathcal{H}(1,2,2,2) = 2$\\
$\mathcal{H}(2,2,2,2) = 2$\\
$\mathcal{H}(1,2,3,3) = 2$\\
$\mathcal{H}(1,3,3,3) = 3$\\
\end{example}

\begin{proposition}
$\mathcal{H}(x_1,x_2,\ldots,x_n) \leq n$
\end{proposition}
\begin{proposition} If $x_i \leq x'_i$ for all integer index $1\leq i\leq n$
$\mathcal{H}(x_1,x_2,\ldots,x_n) \leq \mathcal{H}(x'_1,x'_2,\ldots,x'_n)$
\end{proposition}

We adopt the notion of $\mathcal{H}$-operator~\cite{eugene15} to define Generalised $H$-index.
\begin{definition}[Generalised $H$-index]
The generalised $H$-index of a vertex $i \in V$ of a hypergraph $H = (V,E)$ denoted as $h_i$ is defined as
\[
h_i := \mathcal{H}\left(\abs{N(j_1)},\abs{N(j_1)},\ldots,\abs{N(j_k)}\right)
\]
where $j_1,j_2,\ldots,j_k$ are neighbours of vertex $i$ in hypergraph $H$.
\end{definition}

\begin{definition}[Generalised $H$-index of order $n$]
% \label{def:genHindex} 
The $n$-order Generalised $H$-index of vertex $i \in V$, denoted as $h_i^{(n)}$, is defined for any $n \in \mathbb{N}$ by the recurrence relation
\[ 
    h_i^{(n)}:= 
    \begin{cases} 
      \abs{N(i)} & n=0\\
      \mathcal{H}\left(h^{(n-1)}_{j_1},h^{(n-1)}_{j_2},\ldots,h^{(n-1)}_{j_k}\right) & n \in \mathbb{N}\setminus \{0\}
  \end{cases}
\]
\end{definition}

The number of neighbours of vertex $i$ is its $0$-th order $H$-index. The first-order $H$-index is derived from $\mathcal{H}$-operator applied on the set of neighbours' $0$-th order $H$-indices. The $H$-index of a vertex is precisely its first-order $H$-index, i.e. $h_i^{(1)} = h_i$. Later in~\cref{thm:localconv} we will show that the limiting value of $h_i^{(n)}$ as $n \to \infty$ is the core-number of $i$. One way to interpret this result is that number of neighbours, $H$-index and coreness are respectively the initial, intermediate and steady states under successive operations by $\mathcal{H}$. Given a hypergraph $H = (V, E)$, the convergence time is defined as the minimum number
of iterations required to reach coreness from number of neighbours using the operator $\mathcal{H}$. 

\begin{lemma}
% \label{lem:monotonic}
The sequence $(h_i^{(0)},h_i^{(1)},\cdots,h_i^{(n)},\cdots)$ is monotonically non-increasing for every vertex $i \in V$. 
\end{lemma}
\begin{proof}
We proof that, for any $n \in \mathbb{N}$, $h_i^{(n+1)}  \leq h_i^{(n)}$.
\paragraph{Base case.} Suppose $n = 0$. For any vertex $i \in V$, $h_i^{(1)}$ is the largest integer such that at least $h_i^{(1)}$ elements in $\{ h_{j_1}^{(0)}, h_{j_2}^{(0)},\ldots, h_{j_k}^{(0)} \}$ are no less than $h_i^{(1)}$. $h_i^{1} \leq k$ because there are $k$ elements in set $\{ h_{j_1}^{(0)}, h_{j_2}^{(0)},\ldots, h_{j_k}^{(0)} \}$. But $k = \abs{N(i)} = h_i^{(0)}$. Thus $h_i^{(1)} \leq h_i^{(0)}$ for all $i \in V$.

\paragraph{Inductive case} Suppose for $n = m$, it holds that $h_i^{(n)} \geq h_i^{(n+1)}$ for all $i \in V$. We show that the inequality also holds for $n = m+1$, in other words, $h_i^{(m+1)} \geq h_i^{(m+2)}$ for all $i \in V$.

 $h_i^{(m+2)} = \mathcal{H} \left (h_{j_1}^{(m+1)},h_{j_2}^{(m+1)},\ldots,h_{j_k}^{(m+1)} \right)$ by definition of $\mathcal{H}$-operator and for every neighbour $j$, $h_j^{(m)} \geq h_j^{(m+1)}$ by induction hypothesis. Therefore
 
 \begin{align*}
     h_i^{(m+2)} &= \mathcal{H} \left (h_{j_1}^{(m+1)},h_{j_2}^{(m+1)},\ldots,h_{j_k}^{(m+1)} \right) \\
     &\leq \mathcal{H} \left (h_{j_1}^{(m)},h_{j_2}^{(m)},\ldots,h_{j_k}^{(m)} \right) \\
     &= h_i^{(m+1)}
 \end{align*}

\end{proof}

\begin{lemma}
The sequence $(h_i^{(0)},h_i^{(1)},\cdots,h_i^{(n)},\cdots)$ converges for every vertex $i \in V$.
\end{lemma}
\begin{proof}
For any $n \in \mathbb{N}$, $h_i^{(n)} \geq 0$ by definition of $\mathcal{H}$-operator. Thus  $(h_i^{(0)},h_i^{(1)},\cdots,h_i^{(n)},\cdots)$ is a monotonically  non-increasing sequence (by~\cref{lem:monotonic}) and every element in this sequence is bounded below by $0$ and bounded above by number of neighbours of $i$ (as $h_i^{(0)} = \abs{N(i)}$). By Monotone Convergence Theorem~\cite[p.~104-105]{bartle}, the sequence converges. Let the value it converges to be denoted by $h_i^{\infty}$: 
\[ 
h_i^{\infty} := \lim_{n\to\infty} h_i^{(n)}
\]
\end{proof}

We will require the following two lemmas to prove in~\cref{thm:localconv} that nbr-based core-number is the limiting value of Generalised $H$-index of order $n$. 
\begin{lemma}
If $H' = (V',E')$ is a sub-hypergraph of hypergraph $H = (V,E)$, for any vertex $i \in V'$ the following holds: 
\[
   \forall n  \in \mathbb{N}, h_{i,H}^{(n)} \geq h_{i,H'}^{(n)}
\]
where the subscript $H'$ indicates that the corresponding index is defined on the sub-hypergraph $H'$.
\end{lemma}
\begin{proof}
Since $H'$ is a sub-hypergraph of $H$, the number of neighbours of $i$ in $H'$ can not exceed that in $H$. Thus for $n = 0$, $h_{i,H}^{(n)} = \abs{N_H(i)} \geq \abs{N_H'(i)} = h_{i,H'}^{(n)}$.

Let us assume, as inductive hypothesis, for $n = m$ and vertex $i \in V'$, $h_{i,H}^{(m)} \geq h_{i,H'}^{(m)}$. By inductive hypothesis for any neighbour $j \in V'$ of vertex $i$, $h_{j,H}^{(m)} \geq h_{j,H'}^{(m)}$

If $i \in V'$ has the same number of neighbours ($j_k$) in both $H$ and $H'$, since $h_{j,H}^{(m)} \geq h_{j,H'}^{(m)}$ for any neighbour $j \in \{j_1,j_2,\ldots,j_k\} \subseteq V'$ the following holds:
\begin{align*}
    \mathcal{H}\left(h^{(m)}_{j_1,H},h^{(m)}_{j_2,H},\ldots,h^{(m)}_{j_k,H}\right) 
      &\geq \mathcal{H}\left(h^{(m)}_{j_1,H'},h^{(m)}_{j_2,H'},\ldots,h^{(m)}_{j_k,H'}\right) \\
    h_{i,H}^{(m+1)} \geq h_{i,H'}^{(m+1)}
\end{align*} 
      
If $i \in V'$ has less number of neighbours (say $j_{k'}$) in $H'$ than that in $H'$, since $h_{j,H}^{(m)} \geq h_{j,H'}^{(m)}$ for any $j \in \{j_{1},j_{2},\ldots,j_{k'}\} \subset \{j_1,j_2,\ldots,j_k\} \subseteq V'$,

\begin{align*}
    \mathcal{H}\left(h^{(m)}_{j_1,H},h^{(m)}_{j_2,H},\ldots,h^{(m)}_{j_k,H}\right) 
      &\geq \mathcal{H}\left(h^{(m)}_{j_1,H'},h^{(m)}_{j_2,H'},\ldots,h^{(m)}_{j_{k'},H'}\right) \\
    h_{i,H}^{(m+1)} \geq h_{i,H'}^{(m+1)}
\end{align*} 

Here we used the fact that removal of any element from a set can only reduce if not unchanged its $\mathcal{H}$-operator value along with the observation that $\mathcal{H}$-value of a set with $n$-elements can not exceed $n$.

\end{proof}

\begin{lemma}
If $\mathbf{LB_H}$ is the minimum of the number of neighbours of vertices in hypergraph $H = (V,E)$, for any vertex $i \in V$ the following holds: 
\[
\forall n  \in \mathbb{N}, h_{i}^{(n)} \geq \mathbf{LB_H}
\]

\end{lemma}
\begin{proof}
For $n=0$, $h_i^{(0)} = \abs{N(i)} \geq \min_{j \in V}\,\abs{N(j)} := \mathbf{LB_H}$

Let us assume the statement is true for $n=m$, i.e. $h_{i}^{(m)} \geq \mathbf{LB_H}$. We show that the statement is also true for $n=m+1$. 

By induction hypothesis, for all neighbours $j \in N(i)$, the inequality $h_{j}^{(m)} \geq \mathbf{LB_H}$ holds and there are at least $\mathbf{LB_H}$ such neighbours. Thus there are at least $\mathbf{LB_H}$ elements in set $\{h^m_{j_1},h^m_{j_2},\ldots,h^m_{j_k}\}$ each of which is at least $\mathbf{LB_H}$. By definition of $\mathcal{H}$-operator
\[ 
h_i^{(m+1)} = \mathcal{H}(h^m_{j_1},h^m_{j_2},\ldots,h^m_{j_k}) \geq \mathbf{LB_H}
\]

\end{proof}
\begin{theorem}
% \label{thm:localconv}
For any vertex $i \in V$, its nbr-based core-number $c(i)$ is the limit of its Generalised $H$-index of order $n$ as $n$ tends to $\infty$
\[
    \lim_{n\to\infty} h_i^{(n)} = c(i)
\]
\end{theorem}
\begin{proof} 
Since $h_i^{\infty} = \lim_{n\to\infty} h_i^{(n)}$, it suffices to first show that $h_i^{\infty} \geq c(i)$ followed by showing that $h_i^{\infty} \leq c(i)$.

Let $H' = (V',E') \subseteq H$ be the $c(i)$-core of $H$. Thus $H'$ is a sub-hypergraph containing $i$ where every vertex has at least $c(i)$ neighbours in $H'$. Therefore, $\min_{j \in V'} N_{H'}(j) := LB_{H'}$ must be at least $c(i)$. Applying Lemma 3.10 and Lemma 3.11, 
$\forall n\in \mathbb{N}, h_{i,H}^{(n)} \geq h_{i,H'}^{(n)} \geq LB_{H'} \geq c(i)$. Thus the limit $h_i^{\infty} := \lim_{n \to \infty} h_{i,H}^{(n)} \geq c(i)$.

{\color{red} The following part of the proof may not correct. Because, empirically we found that the core reported for certain vertex $i$ is an overestimate. 

Consider for some given value of $h_i^{\infty}$, $V' = \{j: h_j^{\infty} \geq h_i^{\infty} \}$ and $H[V']$. We expect $H[V'] = h^{\infty}_i$-core. We empirically found that,there are such vertex $j^*$ in $H[V']$- 
\begin{itemize}
    \item although $j^*$ has at least $h^{\infty}_i$-neighbours (in $H$) that are $\geq h^{\infty}_i$,
    \item $j^*$'s number of neighbours in $H[V']$ can be strictly less than $h_i^{\infty}$.
    \item Because some of $j^*$'s neighbours are connected to a `bad' vertex (whose $h^{\infty} < h_i^{\infty}$). Hence those neighbours of $j^*$ are excluded from $h_i^{\infty}$-core (sub-hypergraph).
\end{itemize} 

In general, we needed to show here that $c(i)-core \subseteq h^{\infty}_{i}-core$. 
}

Let $G = (U,E[U]) \subseteq H$ be the $h_i^{\infty}$-core of $H$. Every vertex $l \in U$ including its neighbours $j \in N_{G}(l)$ has at least $h_i^{\infty}$ neighbours in $G$, $\abs{N_{G}(l)} \geq h_i^{\infty}$ and $\forall j \in N_{G}(l)$, $\abs{N_{G}(j)} \geq h_i^{\infty}$. Clearly $i \in G$, because if it had strictly less than $h^{\infty}_{i}$ neighbours, $\mathcal{H}(h^{\infty}_{j_1},\ldots,h^{\infty}_{j_k}) < h_i^{\infty}$ leading to contradiction.

Let us construct another sub-hypergraph $G' = (U',E[U']) \subseteq H$ such that for every $l \in U'$, $h^{\infty}_{l,H} \geq h^{\infty}_{l,G'} \geq h^{\infty}_i$. By definition of $\mathcal{H}$-operator $\mathcal{H}(h^{\infty}_{j_1,G'},h^{\infty}_{j_2,G'},\ldots,h^{\infty}_{j_k,G'}) \geq h^{\infty}_i$. It follows that there must be at least $h_i^{\infty}$ neighbours of $l$ in the sub-hypergraph $G'$ for whom $h^{\infty}_{j,G'} \geq h^{\infty}_i$. Since $G'$ is another sub-hypergraph of $H$ where every vertex $l$ has at least $h_i^{\infty}$ neighbours in $G'$, $G' \subseteq G$. Again $i \in G'$, because  $h^{\infty}_{i,H} = h^{\infty}_{i,G'} = h^{\infty}_i$ satisfying the condition for a vertex to be included in $U'$.

Therefore, $G' \subseteq h^{\infty}_i\text{-core}$ by construction, both sub-hypergraph contains the vertex under consideration $i$, and every vertex $l$ in both sub-hypergraphs has at least $h^{\infty}_i$ neighbours in the respective sub-hypergraph. But $h^{\infty}$-core must be unique (by uniqueness property). Hence $G'$ must be a subset of a higher-order core than $h^{\infty}_i$ or $G' = h
_i^{\infty}\text{-core}$. In the former case $c(i) > h^{\infty}_i$ and in the later case $c(i) = h^{\infty}_i$. Combined together $c(i) \geq h^{\infty}_i$

% Construct subset $U' \subseteq U$ defined as 
% \[ 
% U' := \{ j \in U: h^{\infty}_{j,H} \geq h^{\infty}_{j,G} \geq h_i^{\infty} \}
% \]
% $H[U']$ is a sub-hypergraph of $h_i^{\infty}$-core $G$ such that every vertex has $h^{\infty}$ value at least $h_i^{\infty}$. Clearly $i \in H[U'] \subseteq G$ as well.

% For any $l \in U' \subseteq U$, $h^{\infty}_{l,H} \geq h^{\infty}_{l,G} \geq h_i^{\infty}$ is true. By definition of $\mathcal{H}$-operator, $ \mathcal{H}(h^{\infty}_{j_1,G},\ldots,h^{\infty}_{j_k,G}) \geq h_i^{\infty}$. Hence there must be at least $h_i^{\infty}$ neighbours of $l$ in $G$ for whom the following must hold: $h^{\infty}_{j,H} \geq h^{\infty}_{j,G} \geq h_i^{\infty}$. Hence $H[U']$ is a sub-hypergraph where any vertex has at least at least $h_i^{\infty}$ neighbours in $G$ and $h^{\infty}$ value at least $h^{\infty}_i$

\end{proof}

\begin{theorem}
For any $i \in V$ and iteration $n \in \mathbb{N}$, if $h_i^{(n)}$ is the largest integer such that local coreness constraint is satisfied for $i$ at $h_i^{(n)}$  
\[ 
\hat{h}_i^{(n)} = h_i^{(n)}
\] 
and vice versa.
\end{theorem}
\begin{proof}
Given integer $h_i^{(n)}$ as input (alias $c_u$), ~\cref{alg:core_correct} returns $h_i^{(n)}$ if and only if it finds a suitable sub-hypergraph $(E^+(i), N^+(i))$ at recursion depth $0$ certifying that local coreness constraint is satisfied for $i$ at that integer $h_i^{(n)}$. Thus if local coreness constraint is satisfied for $i$ at $h_i^{(n)}$, line~9 of ~\cref{alg:localcore} guarantees that $\hat{h}_i^{(n)} = h_i^{(n)}$. 

Conversely, If $\hat{h}_i^{(n)} = h_i^{(n)}$, then the algorithm must have made the assignment $\hat{h}_i^{(n)} \gets h_i^{(n)}$ in line~9. Such assignment is only made when Core-Correction module returns at recursion depth $0$. Because otherwise,~\cref{alg:core_correct} would not have terminated at recursion depth $0$, subsequently returning an integer strictly less than $h^{(n)}_i$. Since Core-Correction module returned at recursion depth $0$, local coreness constraint is satisfied  at $h_i^{(n)}$.
\end{proof}

Since we have shown LCC is satisfied for all $i \in V$ when the algorithm terminates, the correctness of the algorithm follows from~\cref{thm:coreconv}.
