# Supplementary material for: Neighborhood-based Hypergraph Core Decomposition
Source: arXiv:2301.06426 source file (2023-04-09)
Supplement: Supplementary file 2 [file appendix_new.tex]

\section{appendix}
\label{appendix}
\spara{Proof of Theorem~\ref{th:unique}.}
Let, if possible, there be two distinct nbr-$k$-cores: $H_{k_1} = (V_{k_1},E[{k_1}])$ and $H_{k_2} = (V_{k_2},E[{k_2}])$ of a hypergraph $H = (V,E)$.
By definition, both $H_{k_1}$ and $H_{k_2}$ are maximal strongly induced subhypergraphs of $H$, induced by $V_{k_1}$ and $V_{k_2}$, respectively.
Construct the union hypergraph $H_k = (V_{k_1} \cup V_{k_2}, E[V_{k_1} \cup V_{k_2}])$. For any $u \in V_{k_1} \cup V_{k_2}$, $u$ must be in either $V_{k_1}$ or $V_{k_2}$.
In both cases, $u$ must have at least $k$ neighbours in the respective subhypergraph $H_{k_1}$ or $H_{k_2}$.
Since $E[V_{k_1}] \cup E[V_{k_2}] \subseteq E[V_{k_1} \cup V_{k_2}]$,
$u$ must have at least $k$ neighbours in $H_k$ as well.
Since $H_k$ is a supergraph of both  $H_{k_1}$ and $H_{k_2}$, $H_k$ is another maximal strongly induced subhypergraph of $H$,
where every vertex $u$ has at least $k$-neighbours. It follows that, $H_{k_1}$ and $H_{k_2}$ are not maximal, and thus are not nbr-$k$-cores,
leading to a contradiction. Hence, it must be that $H_k = H_{k_1} = H_{k_2}$.

\spara{Proof of Theorem~\ref{th:containment}.}
Let, if possible, for some vertex $u \in V_{k+1}$,  $u \notin V_{k}$.
Construct $S=V_{k}\cup V_{k+1}$. Since $u~\notin V_k$, but $u \in V_{k+1} \subset S$, the set $S$ is larger than $V_k$, to be precise, $\abs{S} \geq \abs{V_k} + 1$.

For every $v \in S$: (1) If $v \in V_{k+1}$, $\abs{N_{S}(v)} \geq \abs{N_{V_{k+1}}(v)} \geq k+1 >k$;
(2) if $v \in V_k$, $\abs{N_{S}(v)} \geq \abs{N_{V_k}(v)} \geq k$.
Thus, $S$ is a subset of $V$ where every vertex $v \in S$ has at least $k$ neighbours in $H[S]$ and $S$ is strictly larger than $V_k$. Then, $V_k$ is not maximal and thus not nbr-k-core, which is a contradiction. %The theorem follows.

\spara{Proof of Theorem~\ref{th:refn}}
%\label{sec:proof_th_refn}
Let $V_{k_{max}} \subseteq V$ be the degree-based innermost-core of hypergraph $H$. Thus, $\forall u \in V_{k_{max}}$, its degree-based core number $c^{deg}(u) = k_{max} = \max_{u \in V} c^{deg}(u)$.
%
%We prove by constructing a strongly induced subhypergraph $H[S]$ of $H$,
%such that $\forall u \in S$, its neighborhood-based core number $c(u) \geq {k_{max}}$.
%
Construct $S = V_{k_{max}}$ and the strongly induced subhypergraph $H[S] = (V_{k_{max}},$ $E[V_{k_{max}}])$.
$H[S]$ has the property that every vertex $u \in S$ has at least $k_{max}$ incident hyperedges in $H[S]$.
Each hyperedge must contribute at least one neighbouring vertex (distinct from $u$) to $N_{H[S]}(u)$,
since (1) we focus on hypergraphs consisting of no singleton hyperedges, and
(2) the number of hyperedges between any pair of vertices is no more than one (for this theorem).
Thus, every $u \in S$ has the number of neighbours $\abs{N_{H[S]}(u)} \geq k_{max}$.
%Otherwise, if $\abs{N_{H[S]}(u)} < k_{max}$, by Pigeonhole Principle, there must be some incident hyperedge $e$ that
%contributes zero neighbour to $u$; which contradicts the fact that $\abs{e}>1$.
Therefore, $H[S] = (V_{k_{max}}, E[V_{k_{max}}])$ is a subhypergraph of $H$ such that the following holds:
$\forall u \in S, \abs{N_{H[S]}(u)} \geq k_{max}$.
Since $S \subseteq V$, the maximum of $c(u)$ over $V$ would definitely be at least $\max_{u \in V} c^{deg} (u)$.
%,proving Theorem~\ref{th:refn}.

\spara{Top-Down Algorithm: A Negative Result.}
%\label{sec:top_down}
% \textcolor{red}{this part should go to appendix.}
The \textbf{Top-Down} algorithm~\cite{ChengKCO11,bonchi2019distance} for graph core decomposition uses an upper-bound $UB(v)$ for core number of every vertex $v \in V$ to compute an induced subgraph $G[V]$. It has been shown that for a given value of upper-bound $l$, the computed $G[V']$, where $V'=\{u \in V: UB(u) \geq l \}$, has the following property: \emph{All $k$-cores with $k \geq l$ are contained in $G[V']$} and can be computed from $G[V']$. Based on this property, the algorithm splits the core-computations into a set of sub-computations that are independent from each other. The algorithm computes larger-valued $k$-cores first before proceeding to compute smaller valued $k$-cores. By discovering and peeling the vertices with high core index at earlier stages, the algorithm saves many repeated degree queries.

The above property also holds in hypergraph; however, core numbers computed from $H[V']$ may not be correct. Consider the counter-example in~\Cref{fig:prob1}. Since neighborhood-based core number of a vertex can not exceed its number of neighbors $N(v)$, let us assume the upper-bounding function to be $N(v)$. For a threshold value $l = 3$, the set $V' = \{d,h,c,e,g\}$ because each of these 5 vertices has at least $3$ neighbors in $H$. The induced subhypergraph $H[V']$ is shown in~\Cref{fig:prob2}. Indeed the actual $3$-core is contained in $H[V']$ and the core numbers of vertices $h$,$c$, $e$, and $g$ computed from $H[V']$ are correct. But, the core number of $d$ computed from $H[V']$ is wrong. It is unclear how to identify the vertices whose core numbers are wrongly computed. Even if we can identify such vertices it is not clear how to correct them while computing smaller-valued $k$-cores.
\begin{figure}[!htb]
    \vspace{-2mm}
    \centering
    \begin{minipage}{.45\linewidth}
        \centering
        \includegraphics[width=0.95\linewidth,trim = {1.5cm 1.8cm 0cm 0.5cm},clip]{figures/topdown_baseline.pdf}
        \vspace{-2mm}
        \caption{Hypergraph $H$}
        \label{fig:prob1}
    \end{minipage}
    % \hspace{0cm}
    \begin{minipage}{0.45\linewidth}
        \centering
        \includegraphics[width=0.95\linewidth,trim = {5cm 3.1cm 0cm 1.2cm},clip]{figures/topdown_reduced.pdf}
        \vspace{-2mm}
        \caption{$H[V']$ where $\forall v \in V',~UB(v)=N(v) \geq 3$ }
        \label{fig:prob2}
    \end{minipage}
    \vspace{-3mm}
\end{figure}

\eat{
\spara{Detailed Complexity Analysis of \textbf{Local-core}}
\noindent\emph{Cost of Lines 4-5:} In the worst case, the algorithm needs to compute $\mathcal{H}$-values for all vertices $u \in V$. $\mathcal{H}$-value computation has time complexity $\bigO(\abs{N(u)}\log~\abs{N(u)})$, because any vertex $u \in V$ has $\abs{N(u)}$ neighbors and in the worst-case for all $u \in V$, the set $\{\hat{h}_u^{(n-1)}: u\in N(u)\}$ needs to be sorted to compute $\mathcal{H}$-values. %The worst-case complexity of~lines~4-5 is $O(\sum_u \abs{N(u)}\log~\abs{N(u)})$.

\noindent\emph{Cost of Lines 6-7:} In the worst-case, we may need to correct $h_v^{(n)}$ for all $|V|$ vertices in hypergraph $H$. The cost of correcting a vertex $u \in V$ is $\bigO(d(u)*\abs{(N(u)} - c(u)) = \bigO(d(u)\abs{N(u)})$, where $c(u)$ and $d(u)$ are the actual core number and degree of $u$, respectively. Because in~\Cref{alg:core_correct}, Lines~1-2 traverses all $d(u)$ incident hyperedges of $u$, incurring complexity $\bigO(d(u))$. The recursion-depth (Line~6) is bounded by the discrepancy between the input $h^{(n)}$ at depth $0$ (which is at most $\abs{N(u)}$ for any $n \geq 0$) and the output corrected core value $\hat{h}^{(n)}$ (which is at least $c(u) > 0$). Since such correction might be required for all $u \in V$, the worst-case complexity of~Lines~6-7 is $\bigO(\sum_u d(u)\abs{N(u)}^2)$.
}

\spara{Proof of Theorem 4.}
%\begin{proof}
Construct a new sequence $(h\hat{h}_v)$ by interleaving components from $(h_v^{(n)})$ and $(\hat{h}_v^{(n)})$ as the following:
\begin{small}
\[ (h\hat{h}_v) = (h_v^{(0)}, \hat{h}_v^{(0)},h_v^{(1)}, \hat{h}_v^{(1)},h_v^{(2)}, \hat{h}_v^{(2)}\ldots )
\]
\end{small}
We first show that this \emph{interleave sequence}~\cite[defn~680]{thierry2017handbook}, denoted as $(h\hat{h}_v)$,
is monontonically non-increasing and is lower-bounded by $0$.
Arbitrarily select any pair of successive components from $(h\hat{h}_v)$.

\noindent\textbf{Case 1 $(\hat{h}_v^{(n-1)}, h_v^{(n)})$:} For $n \geq 1$, if $\mathcal{H}\left(\hat{h}_{u_1}^{(n-1)}, \hat{h}_{u_2}^{(n-1)},\ldots,\hat{h}_{u_k}^{(n-1)} \right) > \hat{h}_v^{(n-1)}$, by the recurrence relation (\Cref{eqn:hn}) $h_v^{(n)} = \hat{h}_v^{(n-1)}$. Otherwise, $\hat{h}_v^{(n-1)} \geq \mathcal{H}\left(\hat{h}_{u_1}^{(n-1)}, \hat{h}_{u_2}^{(n-1)},\ldots,\hat{h}_{u_k}^{(n-1)} \right) = h_v^{(n)}$
Here, the equality in the final expression is again due to the recurrence relation \Cref{eqn:hn}. Thus, for any $n \geq 1,~\hat{h}_v^{(n-1)} \geq h_v^{(n)}$.

\noindent\textbf{Case 2 $(h_v^{(n)}, \hat{h}_v^{(n)})$: } For $n = 0$, $h_v^{(0)} = \hat{h}_v^{(0)}$ by ~\Cref{eqn:hhatn}.
For $n>0 \, \land \, LCCSAT(h_v^{(n)})$, again by~\Cref{eqn:hhatn}, $h_v^{(n)} =  \hat{h}_v^{(n)}$.
For $n>0 \, \land \, \neg LCCSAT(h_v^{(n)})$, $\hat{h}_v^{(n)}= \max \{k : k < h_v^{n} \land LCCSAT(k)\} < h_v^{(n)}$.
So, for any $n \geq 0$, irrespective of $LCCSAT(h_v^{(n)})$, $h_v^{(n)} \geq \hat{h}_v^{(n)}$.

Since for any arbitrarily chosen pair of successive components, the left component is not smaller than the right component,
the sequence $(h\hat{h})$ is monotonically non-increasing: $h_v^{(0)} \geq \hat{h}_v^{(0)} \geq h_v^{(1)} \geq \hat{h}_v^{(1)} \geq h_v^{(2)} \geq \hat{h}_v^{(2)} \geq \ldots$

Next, we prove that $h_v^{(n)} > 0$ and $\hat{h}_v^{(n)} > 0$ for all $n \geq 0$ by induction. For $n=0$ due to~\Cref{eqn:hn} and~\Cref{eqn:hhatn}, $h_v^{(0)} = \hat{h}_v^{(0)} = N(v) > 0$. $N(v) > 0$ because the hypergraph is assumed to have no singleton edges and as a result every vertex has at least 1 neighbor. Assume for $n=m$, $h_v^{(m)} > 0$ and $\hat{h}_v^{(m)} > 0$ (induction hypothesis). For $n=m+1$, the recurrence relation for $h_v^{(m+1)}$ is either $\abs{N(v)} > 0$, or output of an $\mathcal{H}$-operator (strictly greater than $0$ by~\Cref{defn:H}), or $\hat{h}_v^{(m)} > 0$ (by induction hypothesis). Considering all three cases: $h_v^{(m+1)} > 0$. For any $n=m+1$ as defined in~\Cref{eqn:hhatn}: $\hat{h}_v^{(m+1)}$ is either $\abs{N(v)} > 0$,
or $h_v^{(m+1)} > 0$ (just proven), or a value $k^* = \max \{k : k < h_v^{(m+1)} \land LCCSAT(k) \}$. By definition of $LCC$ (\Cref{defn:lccsat}), $k^*$ is a value where $N^+(v) \geq k^*$ and $\forall u \in N^+(v), h_u^{(m+1)} \geq k^*$. Consider the set of all hyperedges incident on $v$ ($Incident(v)$) as $E^+(v)$ and $N(v) = (\cup_{e \in Incident(v)} e) \setminus \{v\}$ as $N^+(v)$. Clearly $N(v) = N^+(v)$ contains all neighbors of $v$ and is at least $1$ since the hypergraph is assumed to have no singleton hyperedges. $\forall u \in N(v), h_u^{(m+1)} > 0$ holds as proven in the previous paragraph. Therefore, $k^* \geq 1 > 0$. Considering all three cases: $\hat{h}_v^{(m+1)} > 0$ which completes our proof that the interleave sequence is lower-bounded by $0$.

% For any $n>0$, the recurrence relation for $h_v^{(n)}$ is either $\abs{N(v)} > 0$, or an output of the $\mathcal{H}$-operator (strictly greater than $0$ by~\cref{defn:H}), or $\hat{h}_v^{(n-1)}$.

% For any $n>0$, due to~\cref{eqn:hhatn}, $\hat{h}_v^{(n)}$ is either $\abs{N(v)} > 0$,
% or $h_v^{(n)}$ which we argue to be non-negative, or $max \{k : k < h_v^{(n)} \land LCCSAT(k) \} > 0$.

% Notice that one can always use $k = \mathbf{LB}_1 = \min_{u \in V} \abs{N(u)} > 0$.
% For any $v \in V$, $\mathbf{LB}_1 \leq h_v^{(n)}$ because \textcolor{red}{[AK: the following argument is not clear, how
% it considers the fact for any n? Also, grammatically incorrect and the meaning is not clear]}
% \textcolor{red}{every vertex is no less neighbors than one the least neighbor vertices}.
% Furthermore, $LCCSAT(\mathbf{LB}_1)$ is True because \textcolor{red}{[AK: the following argument is not clear, also
% is Incident() defined?]} \textcolor{red}{for any $v \in V$, $E^+(v) = Incident(v)$ and $N^+(v) = N(v)$ would satisfy
% the condition $\abs{N^+(v)} \geq \mathbf{LB}_1$}.
%% ~\cite[p.~104-105]{bartle}
%% ~\cite[p.~293]{thierry2017handbook}
It follows that $(h\hat{h}_v)$ is monotonically non-increasing and lower-bounded by $0$. By Monotone convergence theorem~\cite{bartle}, $(h\hat{h}_v)$ has a limit. An interleave sequence has a limit if and only if its constituent sequence pairs are convergent
and have the same limit~\cite{thierry2017handbook}. Since $(h\hat{h}_v)$ has a limit,
the sequences $(h_v^{(n)})$ and $(\hat{h}_v^{(n)})$ converges to the same limit:
%\begin{small}
% \[
$\lim_{n \to \infty} h_v^{(n)} = \lim_{n \to \infty} \hat{h}_v^{(n)}$
% \]
% \end{small}
%\end{proof}

\spara{Proof of Theorem 5.}
We use the following lemma for this purpose.

\begin{lem}
\label{lem:LBH}
Let $\mathbf{LB_{H'}}$ be the minimum number of neighbors of any vertex in a subhypergraph $H' = (V',E') \subseteq H$.
Then, for any vertex $v \in V'$, the following holds:
%\begin{small}
%\begin{align}
$\forall n  \in \mathbb{N}, \hat{h}_{v}^{(n)} \geq \mathbf{LB_{H'}}$.
%\end{align}
%\end{small}
\end{lem}

The proof of the Lemma~\ref{lem:LBH} is as follows. 
For $n=0$, $\hat{h}_v^{(0)} = \abs{N(v)} \geq \min_{u\in V}\,\abs{N_{V'}(u)} = \mathbf{LB_{H'}}$

Let us assume the statement to be true for $n=m$, i.e., $\hat{h}_{v}^{(m)} \geq \mathbf{LB_{H'}}$ for all $v \in V$. We show that the statement is also true for $n=m+1$.

If $LCCSAT(h_v^{(m+1)})$ is true, by definition of $\hat{h}_v^{(n)}$, either  $\hat{h}_v^{(m+1)} = h_v^{(m+1)}$ $= \hat{h}_v^{(m)} \geq LB_{H'}$ (by induction hypothesis) or
$\hat{h}_v^{(m+1)} = h_v^{(m+1)} =  \mathcal{H}\left(\hat{h}^{(m)}_{u_1},\hat{h}^{(m)}_{u_2},\ldots,\hat{h}^{(m)}_{u_k}\right)$. Here $u_1,\ldots,u_k$ are the neighbors of $v$ in $H$.  if $v$ is not the vertex which has exactly $LB_{H'}$ neighbors then $\abs{N_H'(v)} \geq LB_{H'}$, otherwise $\abs{N_H'(v)} = LB_{H'}$. In both cases, $k \geq \abs{N_H'(v)} \geq LB_{H'}$ because $v$ originally had $k$ neighbors and in the subhypergraph $H'$ that number can only decrease.
% Total number of numbers of $v$ in $H$ must be at least the number of neighbors $v$ has in sub-hypergraph $H'$ \textcolor{red}{[AK: not clear]}:
Among those $k$ neighbors, any neighbor $u$ that is also in $H'$, satisfies $h_u^{(m)} \geq LB_{H'}$. Thus $\mathcal{H}$-value $\mathcal{H}\left(\hat{h}^{(m)}_{u_1},\hat{h}^{(m)}_{u_2},\ldots,\hat{h}^{(m)}_{u_k}\right) \geq LB_{H'}$. Considering all cases, $\hat{h}_v^{(m+1)} \geq LB_{H'}$.

If $\neg LCCSAT(h_v^{(m+1)})$, $\hat{h}_v^{(m+1)}$ is the largest integer smaller than $h_v^{(m+1)}$ such that $LCC(\hat{h}_v^{(m+1)})$ is True. In other words, $\hat{h}_v^{(m+1)}$ is such an integer that at least $\hat{h}_v^{(m+1)}$ neighbors of $v$ must satisfy $h_u^{(m+1)} \geq \hat{h}_v^{(m+1)}$. But $LB_{H'}$ is another integer such that at least $LB_{H'}$ neighbors of $v$, in particular any  $u\in N(v) \in H'$ satisfies $h_u^{(m+1)} \geq LB_{H'}$: because by~\Cref{eqn:hn} either $h_u^{(m+1)} = \hat{h}_u^{(m)} \geq LB_{H'}$ (inductive hypothesis applied on $u$) or  $h_u^{(m+1)} = \mathcal{H}\left(\hat{h}^{(m)}_{u_1},\hat{h}^{(m)}_{u_2},\ldots,\hat{h}^{(m)}_{u_k}\right) \geq LB_{H'}$ by an argument similar to that in the previous paragraph. Therefore, $\hat{h}_v^{(m+1)} \geq LB_{H'}$ because clearly for $k = LB_{H'}$ it holds that $\hat{h}_v^{(m+1)} \geq LB_{H'}$.

\underline{Proof of Theorem 5.}
Since $LCCSAT(\hat{h}_v^{\infty})$ holds for vertex $v$, there exists a subhypergraph $H^+(v) = (N^+(v), E^+(v)) \subseteq H$ containing at least $\hat{h}_v^{\infty}$ neighbors of $v$ such that every one of those neighbors $u\in N^+(v)$ satisfies $\hat{h}_u^{\infty} = h_u^{\infty} \geq \hat{h}_v^{\infty}$. We first show that $c(v) \geq \hat{h}_v^{\infty}$. Let us construct a new hypergraph $H^+[N'] \subseteq H$ where $N'$ is constructed by taking union of $N^+(v)$ and all other sets $N^+(w)$ such that $\hat{h}_w^{\infty} \geq \hat{h}_v^{\infty}$ for $w \neq v$:
% \begin{small}
% \[
$N' = N^+(v) \cup \cup_{w \in V} \{N^+(w)\mid \hat{h}_w^{\infty} \geq \hat{h}_v^{\infty}\}$.
% \]
% \end{small}
For any $u\in N'$, $w \in N^+(u)\implies w \in N'$ because by construction of $(N^+(u),E^+(u))$, $w \in N^+(u)$ implies $\hat{h}_{w}^{\infty} \geq \hat{h}_u^{\infty} \geq \hat{h}_v^{\infty}$. Therefore, $N^+(w)$ must be one of the sets used for constructing $N'$ via union operator: $N^+(w) \subseteq N'$. By definition of LCC, $u$ has at least $\abs{N^+(u)} \geq \hat{h}_v^{\infty}$ such neighbors in $N^+(u)$. Since for any $u\in N'$, $w \in N^+(u)\implies w \in N'$ and there are at least $\hat{h}_v^{\infty}$ such vertex in $N'$, every vertex in $H^+[N']$ has at least $\hat{h}_v^{\infty}$ neighbors in $H^+[N']$. Since $\hat{h}_v^{\infty}$-core is the maximal subhypergraph where every vertex has at least $\hat{h}_v^{\infty}$ neighbors in that subhypergraph, $H^+[N']$ is a subhypergraph of $\hat{h}_v^{\infty}$-core: $H^+[N'] \subseteq \hat{h}_v^{\infty}$-core. By definition of core number, $c(v)$ is the largest integer for which $v \in c(v)$-core. Thus, $c(v) \geq \hat{h}_v^{\infty}$. Finally, let the $c(v)$-core be $H'$. Let $LB_{H'}$ be the minimum among the numbers of neighbors of vertices in $H'$. By definition, $LB_{H'} = \min_{u\in H'} \abs{N_{H'}(u)}$. Since every vertex $u$ in $c(v)$-core has at least $c(v)$ neighbors in that core: $\abs{N_{H'}(u)} \geq c(v)$ for any $u\in H'$. Therefore, $LB_{H'} = \min_{u\in H'} \abs{N_{H'}(u)} \geq c(v)$. Since $v \in H' \subseteq H$, applying~\Cref{lem:LBH}: $\hat{h}_v^{(n)} \geq LB_{H'} \geq c(v)$ for any $n \in \mathbb{N}$. Thus, $\hat{h}_v^{\infty} = \lim_{n \to \infty} \hat{h}_v^{(n)} \geq c(v)$.

\eat{
\spara{Algorithm 5: Finding Densest Subhypergraph.}
%\label{sec:alg_approx}
%
%Inspired by Charikar~\cite{charikar},
We design Algorithm~\ref{alg:approx} for (approximate) volume-densenst
subhypergraph detection.
} 
%This follows the peeling paradigm: In each round,
%it removes the vertex which has the smallest number of neighbors in the
%current subhypergraph (Lines 2-4), and we finally return the subhypergraph
%that achieves the largest volume-density (Line 5).
%
\begin{algorithm}[!tb]
\caption{Approximate volume-densest subhypergraph detection}
\label{alg:approx}
\begin{algorithmic}[1]
\scriptsize
\Require Hypergraph $H = (V,E)$
\Ensure Hypergraph $H^*$
\State $S_1 \gets V$
\For{$i \gets 1,2,\ldots,n-1$}
    \State $u_i \gets \argminG_{u\in S_i} \abs{N_{S_i}(u)}$
    % \Comment{$N(u)\at{S_i}$is the set of neighbors of $u$ in $(S_i,E[S_i])$}
    \State $S_{i+1} \gets S_i \setminus \{u_i\}$
\EndFor
\State $H^* \gets \argmaxG_{\{H[S_i]\mid i \in [n]\}} \rho^N[S_i]$
\State \textbf{return} $H^*$
\end{algorithmic}
\vspace{2mm}
\end{algorithm}
%
% \subsection{Additional Experimental Results}
% \label{sec:additional_exp}
%
% \paragraph{Memory Usage}
% We analyze the memory taken by \textbf{Peel}, \textbf{E-Peel}, and \textbf{Local-core}
% algorithms in Figure~\ref{fig:memory}. For each algorithm, we report the maximum memory
% consumed during their execution. We find that the \textbf{Local-core} algorithm
% consumes the least amount of memory, and both \textbf{Peel} and \textbf{E-Peel} algorithms
% take almost similar amount of memory. Thus, \textbf{Local-core} is not only efficient
% in terms of execution time, but is also efficient in memory usage.
% %
% \begin{figure}
% 	\centering
% 	\subfloat[Small dataset]{\includegraphics[scale=0.25]{figures/small_memory_taken.pdf}}
% 	\subfloat[Large dataset]{\includegraphics[scale=0.25]{figures/large_memory_taken.pdf}}
%     \vspace{-2mm}
% 	\caption{Memory footprints of different algorithms}
% 	\label{fig:memory}
%     \vspace{-4mm}
% \end{figure}

\spara{Datasets.}
%We generate three synthetic datasets: \emph{bin4U}, \emph{bin3U}, and \emph{pref3U}.
{\em bin4U} and {\em bin3U} are $4$-uniform and $3$-uniform hypergraphs. Both of their degree sequences follow binomial distribution with $n = 500$ and $p = 0.2$~\cite{arafat2020construction}.
{\em pref3U} is a $3$-uniform hypergraph generated using preferential-attachment model~\cite{avin2019random}
with parameters $p = 0.5$ and $k = 3$, where $p$ is the probability of a new vertex being preferentially attached to current hypergraph and $k$ is the uniform cardinality.
%The degree distribution of \emph{pref3U} approximately follows power-law with exponent $\beta = 2.2$~\cite{avin2019random}. 
%We consider four real-world datasets: \emph{enron}, \emph{contact}, \emph{congress}, and \emph{dblp}. 
{\em Enron} is a hypergraph of emails, where each email correspondence is a hyperedge and users are vertices \cite{benson2018simplicial}. We derive {\em contact} (in a school) dataset from a graph where each maximal clique is viewed as a hyperedge and individuals are vertices~\cite{benson2018simplicial}. In the {\em congress} dataset, vertices are congress-persons and each hyperedge comprises of sponsors and co-sponsors (supporters) of a legislative bill put forth in both the House of representatives and the senate ~\cite{benson2018simplicial}. In {\em dblp} hypergraph, vertices are authors and a hyperedge consists of authors in a publication recorded on DBLP~\cite{benson2018simplicial}.

\spara{Applications in Information Diffusion.}
%\label{sec:exp_applications}
% \subsubsection{Case Studies}
% \textbf{Objective}: Illustrate that innermost core in a real-scenario has applied meaning in that domain.
We empirically study the significance of vertices in the innermost core of a hypergraph derived from neighborhood-based core decomposition.
% To this end, %we apply a diffusion modeling algorithm~\cite{kitsak} on a hypergraph and study the practical impact of vertices belonging to the innermost core. More specifically,
We consider the \emph{SIR} diffusion process~\cite{kitsak}, where initially all vertices except one\textemdash called a \textit{seed}\textemdash are at the \emph{susceptible} state. The seed vertex is initially at the \emph{infectious} state. At each time step, each infected vertex infects its susceptible neighbors %in the hypergraph 
with probability $\beta$ and then enters into \emph{immunized} state. Once a vertex is immunized, it is never re-infected.

\underline{Innermost core contains influential spreaders.}
Our first hypothesis is to understand whether vertices with higher core numbers are highly-influential spreaders.
We compute core-numbers of vertices in {\em enron}. we randomly select a seed vertex from each core-number and run the {\em SIR} model with $ \beta$ = 0.3. Finally, we compute the number of infected vertices after 100 time-steps. We repeat this process 100 times
and report the average number of infected vertices in Figure~\ref{fig:application}(a). We observe that innermost core vertices infect a larger part of the
population compared to outermost core vertices irrespective of decomposition types. 

% We also observe that seeds selected following degree-based decomposition does not exhibit this phenomenon as consistently as those
% selected following neighborhood-based decomposition.

%
%\textcolor{red}{Redundant: We empirically validate epidemic spreading efficacy by running SIR hypergraph-diffusion model with an innermost-core vertex as seed vertex $u_s$. Since neighborhood based innermost-core is different from degree-based innermost-core, we vary seed vertex and measure the following quantity:
%	\[
%	I(k) = \frac{1}{\abs{V_k}} \sum_{u_s \in V_k} \frac{Infected(u_s, \tau)}{|V|}
%	\]
%	Here $V_k$ indicates the set of vertices in $k$-core $H[V_k] = (V_k,E[V_k])$, $Infected(u_s, \tau)$ indicates the number of vertices in the hypergraph infected after $\tau$ time-step when the epidemic diffusion starts from seed vertex $u_s \in V_k$. Intuitively, $I(k)$ measures the expected proportion of infected population if diffusion starts from a vertex chosen from $k$-core uniformly at random.
%}
%\input{sections/epidemic_1}

\begin{figure}
    \vspace{-3mm}
    \centering
    % \subfloat{\includegraphics[scale=0.2]{appl_figs/enron_03_propagation_mean_all_algo.pdf}}
    \subfloat{\includegraphics[scale=0.2]{appl_figs/enron_03_propagation_mean_ours.pdf}}
    \subfloat{\includegraphics[scale=0.2]{appl_figs/naive_nbr_enron_03_propagation_exp2.pdf}}
    %\subfloat{\includegraphics[scale=0.33]{appl_figs/naive_degree_enron_03_propagation_exp2.pdf}}
    % \subfloat[][Congress]{\includegraphics[scale=0.33]{appl_figs/naive_nbr_congress_03_propagation_mean.pdf}}
    % \subfloat[][Contact]{\includegraphics[scale=0.33]{appl_figs/naive_nbr_contact_03_propagation_exp2.pdf}}
    \vspace{-3mm}
    \caption{\small Effect of the core number on information diffusion over {\em enron}. (a) The number of infected vertices increases as the core number of the seed node increases. (b) The first infection time of vertices decreases for vertices with higher core numbers indicating innermost cores are infected earlier.} % \textcolor{red}{Neighborhood-based core-numbers gives a more fine grained decomposition of vertices depending on their first infection-time compared to degree-based decomposition.}
    \label{fig:application}
    \vspace{-4mm}
\end{figure}
\begin{figure}
    \centering
     \subfloat[]{\includegraphics[scale=0.25]{appl_figs/enron_03_propagation_intervention2.pdf}}
    \subfloat[]{\includegraphics[scale=0.25]{appl_figs/Explain_enron_intervention.pdf}}
    \caption{\small (a) Effectiveness of core-decomposition based intervention strategy on Enron dataset. (b) The number of vertices reachable from a seed vertex reduces as innermost cores are deleted.}
    \label{fig:appl3}
\end{figure}
\underline{Innermost core contains early adopters.}
Our second hypothesis is whether vertices in the innermost core are contracts infection early. We select a seed vertex from the hypergraph uniformly at random and run the {\em SIR} model for 100 time-steps. For each seed vertex, we record the time-step at which other vertices are infected. Repeating 1000 times with different seeds, we report the average first infection-times.  Figure~\ref{fig:application}(b) indicates that vertices in inner-cores are infected earlier than those in outer-cores.

\underline{A diffusion-intervention strategy based on core-decomposition.} As core-numbers have significant impact on number of infected population, can we develop an intervention strategy to mitigate diffusion? 

We propose the following intervention strategy: \emph{delete the vertices in the innermost core along with the hyperedges strongly-induced by those vertices.} In order to measure the effectiveness of this strategy, we measure the number of infected population before and after innermost core is deleted. We expect the number of infected population to reduce after intervention. 

\Cref{fig:appl3}(a) shows the effectiveness of our intervention strategy on Enron dataset. $H0 = H$ is the input hypergraph. $H1$ is constructed by deleting vertices in the innermost core of $H0$, $H2$ is constructed by deleting vertices in the innermost core of $H1$, and so on. The number of infected population generally decreases irrespective of the origin of infection. Because deleting innermost core reduces the number of vertices reachable from a seed vertex (component size) as shown in~\cref{fig:appl3}(b). Indeed the vertices that are reachable from a seed vertex, may no longer be reachable after deletion of the innermost-core. 

%We observe a similar trend for degree-based core decomposition in the rightmost plot in Figure~\ref{fig:application}. However, the neighborhood-based approach results in a smoother graph than the degree-based approach, specially when the core number is higher where degree-based approach shows a higher variance.

\paragraph{Effectiveness of neighborhood-based core decomposition compared to other approaches.} \naheed{Reduction in infected population due to using nbr-core based intervention is greater than that using degree-based core decomposition. @Bishwa}

%\vspace{-1.5mm}
\section{Related Work}
\label{sec:related}
Recently, there has been a growing interest in hypergraph data management \cite{SybrandtSS22,FenderM13,WhangDJLDLKP20,KabiljoKPPSAP17,LeeKS20,shun2020practical}.
%, such as
%join enumeration for hypergraphs \cite{FenderM13},
%clustering \cite{WhangDJLDLKP20,AmburgVB20,KamhouaZ0CLH21}, sampling \cite{ChoeYLBKS22},
%betweenness centrality \cite{LeeK17}, community discovery \cite{BrinkmeierWR07},
%hypergraph partitioning \cite{KabiljoKPPSAP17,SybrandtSS22}, subhypergraph matching \cite{9739081},
%hyperedge prediction~\cite{kijung},
%hypergraph neural networks \cite{0004RZLY22,ZhangWCZWZ020,FengYZJG19}, motifs~\cite{LeeKS20,LeeS21},
%hypergraph null models for the purpose of hypergraph property estimation~\cite{arafat2020construction,chodrow},
%as well as parallel algorithms for computing those properties~\cite{shun2020practical}.
As we focus on core decomposition, we 
%urge readers with a much broader interest to 
refer to
recent surveys~\cite{tina21,giovanni20,Eliassi-RadLRS21,Lee22} for a general exposition.

\spara{Core decomposition in hypergraphs.}
%Although core decomposition of graphs has been studied for decades \cite{Malliaros20}, 
There are relatively few works on
hypergraph core decomposition. Ramadan et al.~\cite{ramadan2004hypergraph} propose a peeling
algorithm to find the maximal-degree based $k$-core of a hypergraph.
%They define $k$-core as the maximal subhypergraph where every vertex has maximal-degree at least $k$. Maximal degree of a vertex is the number of hyperedges incident on that vertex such that none of the hyperedges counted for degree are subsets of each other.
%Jiang et al.~\cite{jiang2017parallel} study parallel peeling process on random $k$-uniform hypergraphs and derive
%lower bound on the number of random peelings required until an empty core is found with high probability.
~\cite{jiang2017parallel,shun2020practical} discuss parallel implementations of degree-based hypergraph core computation
based on peeling approach. Sun et al.~\cite{sun2020fully} propose a fully dynamic approximation
algorithm that maintains approximate degree-based core-numbers of an unweighted hypergraph.
%under insertion and deletion of edges.
Gabert et al.~\cite{GabertPC21}
study degree-based core maintenance in dynamic hypergraphs,
and propose a parallel (shared-memory) local algorithm.
None of these works explore our neighborhood-based
hypergraph core decomposition, which is different from degree-based hypergraph core computation (\S \ref{sec:intro}). The existing approaches for degree-based core decomposition cannot be easily adapted for neighborhood-based hypergraph core computation (\S \ref{sec:algorithm}). 
%, nor do they consider algorithmic approaches other than peeling.

\spara{Core decomposition in graphs.} %Graph core decomposition has been used in
%many applications, including dense subgraph discovery \cite{charikar,AC09}, speeding up community search
%\cite{SG10}, graph clustering \cite{Giatsidis14}, and maximal cliques finding \cite{E10},
%identifying influential spreaders \cite{RePE}, %network visualization \cite{Alvarez-HamelinDBV05},
%chromatic number \cite{M83},
%engagement in social networks \cite{B15}, location-based \cite{KimGFCKC20},
%protein interaction \cite{Altaf03}, and brain networks analysis \cite{HagmannEtAl2008}.
The linear-time peeling algorithm for graph core decomposition \cite{Malliaros20} was given by Batagelj and Zaver{\v{s}}nik \cite{Batagelj11}.
Core decomposition has also been studied in disk-based \cite{ChengKCO11,K15},
distributed \cite{distributedcore,SariyuceSP18}, parallel \cite{D17}, and streaming \cite{S13} settings, and
for varieties of graphs, e.g., weighted \cite{al2017identification,Zhou0HY0021}, directed \cite{LiaoLJHXC22},
temporal \cite{GalimbertiCBBCG21}, uncertain \cite{FGKV14}, and multi-layer \cite{GalimbertiBGL20} networks.
Higher-order cores in a graph (e.g., $(k,h)$-core \cite{bonchi2019distance,LiuZHX21}, triangle $k$-core \cite{ZhangP12},
$h$-clique-core, pattern-core \cite{Tsourakakis15a,FYCLX19}) and more complex cores in an attributed network
(e.g., meta-path-based core \cite{FangYZLC20} and $(k,r)$-core \cite{ZhangZQZL17})
have been proposed. In \S \ref{sec:diff}, we reasoned that existing approaches for graph core decomposition
cannot be easily adapted for neighborhood-based hypergraph core decomposition. We also depicted
that the local approach \cite{distributedcore,eugene15}, an efficient method for graph core decomposition,
produces incorrect core-numbers for neighborhood-based hypergraph core decomposition (\S \ref{sec:local}, \S \ref{sec:experiments}).
